# Supplementary material for: Maximizing Welfare in Social Networks under a Utility Driven Influence Diffusion Model
Source: arXiv:1807.02502 source file (2019-05-30)
Supplement: Supplementary file 1 [file appendix.tex]

\clearpage

\appendix

\section{Inductive Proof for the MIA model}

Initial condition, when the depth of node $v$ is zero (i.e. the node is a leaf):

\begin{itemize}
\item
If $v\in S_A \cap S_B$, then $\ap_{AB}(v) = 1$, and $\ap_{A\bar{B}}(v) = 
	\ap_{\bar{A}B}(v) = \ap_{\bar{A}\bar{B}}(v)=0$.
	
\item
If $v\in S_A \setminus S_B$, then $\ap_{A\bar{B}}(v) = 1$, and
	$\ap_{AB}(v) = \ap_{\bar{A}B}(v) = \ap_{\bar{A}\bar{B}}(v)=0$.

\item
If $v\in S_B \setminus S_A$, then $\ap_{\bar{A}B}(v) = 1$, and
	$\ap_{AB}(v) = \ap_{A\bar{B}}(v) = \ap_{\bar{A}\bar{B}}(v)=0$.

\item
If $v \not \in S_A \cup S_B$, then $\ap_{\bar{A}\bar{B}}(v) = 1$, and
	$\ap_{AB}(v) = \ap_{A\bar{B}}(v) = \ap_{\bar{A}B}(v)=0$.
\end{itemize}

For internal node $v$, i.e., depth at least $1$, we have the following recursion.
For convenience, we consider that there is no seeds in the internal nodes first. 
We first have the formulas for informing probabilities:
\begin{align}
\ip_{A\bar{B}}(v,j) =\, & \ip_{A\bar{B}}(v,j-1) (1 - \ap_B(u_j) p_{u_j, v} ) \nonumber \\
	& + \ip_{\bar{A}\bar{B}}(v, j-1) \, \ap_{A\bar{B}}(u_j) \, p_{u_j, v};  \label{EQN:IP-Aapp} \\
\ip_{\bar{A}B}(v,j)  =\, & \ip_{\bar{A}B}(v,j-1) (1 - \ap_A(u_j) p_{u_j, v} ) \nonumber \\
	& + \ip_{\bar{A}\bar{B}}(v, j-1) \, \ap_{\bar{A}B}(u_j) \, p_{u_j, v}; \label{EQN:IP-Aapp} \\
\ip_{AB}(v,j) =\, &(1-p_{u_j, v})\ip_{AB}(v, j-1) + p_{u_j, v} (\ap_{AB}(u_j)  \nonumber\\
	&	+ \ap_{A\bar{B}}(u_j) \ip_{B}(v,j-1) +  \ap_{\bar{A}B}(u_j) \ip_{A}(v,j-1) \nonumber\\
	& + \ap_{\bar{A}\bar{B}}(u_j) \ip_{AB}(v,j-1)); \\
\ip_{\bar{A}\bar{B}}(v,j) =\, &\ip_{\bar{A}\bar{B}}(v, j-1)
	(1-p_{u_j, v} + p_{u_j, v} \ap_{\bar{A}\bar{B}}(u_j) ).
\end{align}
Then the formulas for the adoption probabilities:
\begin{align}
\ap_{A\bar{B}}(v) =\, & \ip_{A\bar{B}}(v) \, \qao + \ip_{AB}(v) \, \qao \, (1-\qba); \label{EQN:AP-Aapp} \\
\ap_{\bar{A}B}(v) =\, & \ip_{\bar{A}B}(v) \, \qbo + \ip_{AB}(v) \, \qbo \, (1-\qab); \label{EQN:AP-Bapp} \\
\ap_{AB}(v)	=\, & \ip_{AB}(v) \, (\qao \, \qba + \qbo \, \qab - \qao \, \qbo); \\
\ap_{\bar{A}\bar{B}}(v) =\, & \ip_{\bar{A}\bar{B}}(v) + \ip_{A\bar{B}}(v) (1-\qao) 
		+ \ip_{\bar{A}B}(v)(1-\qbo) \nonumber \\
	& + \ip_{AB}(v)(1-\qao)(1-\qbo).
\end{align}

\begin{lemma}
Suppose the depth of node $v$ is $d$. 
If we increase $\qao$ to $\qao' = c\qao$ with $1< c \le \qab/\qao$, then we have:
\begin{align*}
& \ip_{AB}(v,j) \le \ip_{AB}'(v,j) \le c^{d-1} \ip_{AB}(v,j),   \\
& \ip_{A\bar{B}}'(v,j) \le c^{d-1} \ip_{A\bar{B}}(v,j),  \\
& \ip_{\bar{A}B}'(v,j) \le \ip_{\bar{A}B}(v,j), \\
& \ip_{\bar{A}\bar{B}}'(v,j) \le \ip_{\bar{A}\bar{B}}(v,j),  \\
& \ip_{\bar{B}}'(v,j) \le \ip_{\bar{B}}(v,j),  \\
& \ap_{AB}(v,j) \le \ap_{AB}'(v,j) \le c^{d} \ap_{AB}(v,j),   \\
& \ap_{A\bar{B}}'(v,j) \le c^{d} \ap_{A\bar{B}}(v,j),  \\
& \ap_{\bar{A}B}'(v,j) \le \ap_{\bar{A}B}(v,j), \\
& \ap_{\bar{A}\bar{B}}'(v,j) \le \ap_{\bar{A}\bar{B}}(v,j),  \\
& \ap_{\bar{B}}'(v,j) \le \ap_{\bar{B}}(v,j).
\end{align*}
\end{lemma}
\begin{proof}
We prove by induction on the depth $d$.
When $d=0$, the adoption probabilities are fixed and are not affected by $\qao$, so
	all inequalities hold for adoption probabilities hold.
When $d=1$, the informing probabilities are only determined by the adoption
	probabilities in the previous level, so are also fixed, not affected by $\qao$.
Thus the base case holds.

For the induction step, we assume that the adoption probability inequalities hold 
	for depth $d-1$ and the informing probability inequalities hold for depth $d$,
	for $d\ge 1$,
	and we will prove that adoption probability inequalities hold for depth $d$ and
	the informing probability inequalities hold for depth $d+1$.
	
We first check adoption probability inequalities one by one.
\begin{align*}
\ap_{AB}'(v) =\, & \ip_{AB}'(v) \, (\qao' \, \qba + \qbo \, \qab - \qao' \, \qbo) \\
\le\, & c^{d-1} \ip_{AB}(v) \, (c\qao (\qba-\qbo) + \qbo \, \qab) \\
\le\, & c^{d} \ip_{AB}(v) \, (\qao (\qba-\qbo) + \qbo \, \qab) \\
= \, & c^{d} \ap_{AB}(v).
\end{align*}
\begin{align*}
\ap_{AB}'(v) =\, & \ip_{AB}'(v) \, (\qao' \, \qba + \qbo \, \qab - \qao' \, \qbo) \\
\ge\, & \ip_{AB}(v) \, (c\qao (\qba-\qbo) + \qbo \, \qab) \\
\ge\, & \ip_{AB}(v) \, (\qao (\qba-\qbo) + \qbo \, \qab) \\
= \, & \ap_{AB}(v).
\end{align*}
\begin{align*}
\ap_{A\bar{B}}'(v) =\, & \ip_{A\bar{B}}'(v) \, \qao' + \ip_{AB}'(v) \, \qao' \, (1-\qba)  \\
\le \, & c^{d-1} \ip_{A\bar{B}}(v) \, c\qao + c^{d-1}\ip_{AB}(v) \, c\qao \, (1-\qba) \\
= \, & c^d \ap_{A\bar{B}}(v).
\end{align*}
\begin{align*}
\ap_{\bar{A}B}'(v) =\, & \ip_{\bar{A}B}'(v) \, \qbo + \ip_{AB}'(v) \, \qbo \, (1-\qab) \\
\end{align*}
\weic{Here, we seems to need 
\[ \ip_{\bar{A}B}'(v) + \ip_{AB}'(v) \, (1-\qab) \le \ip_{\bar{A}B}(v) + \ip_{AB}(v) \, (1-\qab). \]}

\begin{align*}
\ap_{\bar{A}\bar{B}}'(v) =\, & \ip_{\bar{A}\bar{B}}'(v) + \ip_{A\bar{B}}'(v) (1-\qao') 
		+ \ip_{\bar{A}B}'(v)(1-\qbo) \\
	& + \ip_{AB}'(v)(1-\qao')(1-\qbo)
\end{align*}
\weic{Here, we also seem to need more assumptions. Not sure if there is a clean way to proceed
with the inductive proof.
It looks like we need some combination of inequalities, but one has to work very hard to discover
all necessary inequalities and inductively prove all of them.}
\end{proof}
