# Supplementary material for: Maximizing Welfare in Social Networks under a Utility Driven Influence Diffusion Model
Source: arXiv:1807.02502 source file (2019-05-30)
Supplement: Supplementary file 2 [file sec-appendix.tex]

\begin{theorem}\label{thm:val_nonmonotone}
Expected adoption is not self monotone under local noise, for an arbitrary value function.
\end{theorem}
\begin{proof}

\begin{figure}[h]
  \includegraphics[width=0.5\textwidth]{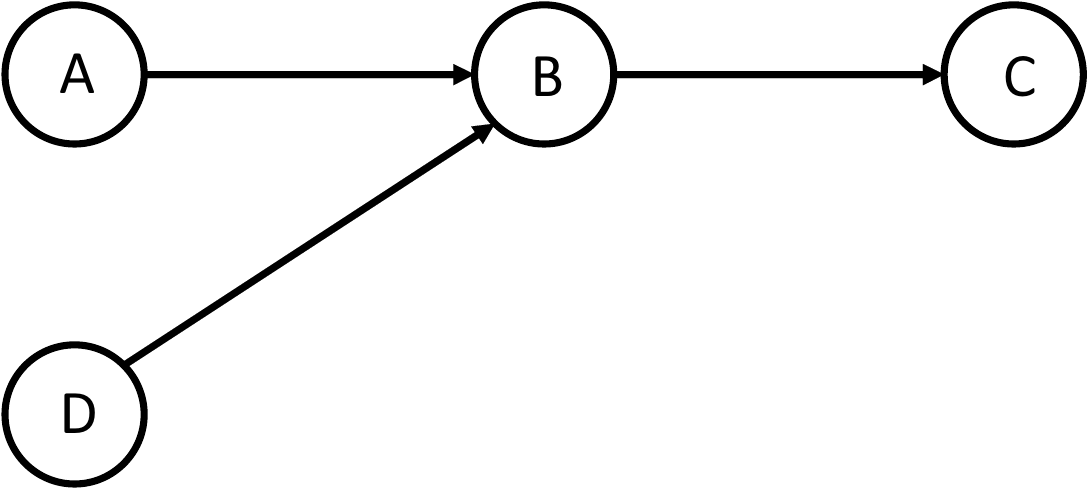}
  \caption{Network for general value function}
  \label{fig:non_monotone}
\end{figure}

Consider Figure~\ref{fig:non_monotone}. All edge probabilities are assumed to be $1$ in the graph. Assume there are three items in propagation, $i_1,i_2$ and $i_3$. Let the value and price function be such that the deterministic utilities for any node satisfy the following: 
$\util^D(\{j,k\}) >\util^D(\{i,j\}) > \util^D(\{i,k\})> \util^D(\{i,j,k\}) >\util^D(j) >\util^D(i) >0 >\util^D(k).$
Let us now consider monotonicity the w.r.t. item $i_1$. Assume two seed allocations be $\allseeds^1 = \{(A,i),(A,j), (E, k)\}$ and $\allseeds^2 = (A,i),(A,j),(E,i),(E,k)\}$. Thus $S_{i}^1 = \{(A,i)\}$, in $\allseeds^1$ and $S_{i}^2 = \{(A,i),(E,i)\}$, in $\allseeds^2$. Whereas, $S_{-i}^1 = S_{-i}^2 = \{(A,j),(E,k)\}$.

Let $\sigma_i(\allseeds,t)$, denote the number of $\Item$ adopted nodes, for seed allocation $\allseeds$ at time $t$.  

\noindent 
\textbf{Cascade under $\allseeds^1$}: At time $t=1$ the expected nodes adopting $i$ is $A$. At $t=2$, $A,B$ and at $t=3$ it is $A,B,C$. There will no more adoption after $t=3$. Thus $\sigma_{i}(\allseeds^1) = 3$.  

\noindent 
\textbf{Cascade under $\allseeds^2$}: At time $t=1$ expected adoption of $i$ is $A, E$. However at time $t=2,3$, no other node adopts $i$. Thus $\sigma_{i}(\allseeds^2) = 2$. The reason for this decrease is that the expected utility of adopting $j$ and $k$ is more than $i$. Thus the introduction of additional seed boosts the utility of item $k$. Thus $k$ gets introduced in the network, which in turn produces more utility than $i$ with presence of other items. Thus the adoption of $i$ decreases. 
\end{proof}

\begin{theorem}\label{thm:max_nonmonotone}
Expected adoption is not self monotone under local noise, when the value function is $max$.
\end{theorem}

\begin{proof}

Consider a network as shown in figure \ref{fig:max_with_noise}.
\begin{figure}[h]
  \includegraphics[width=0.5\textwidth]{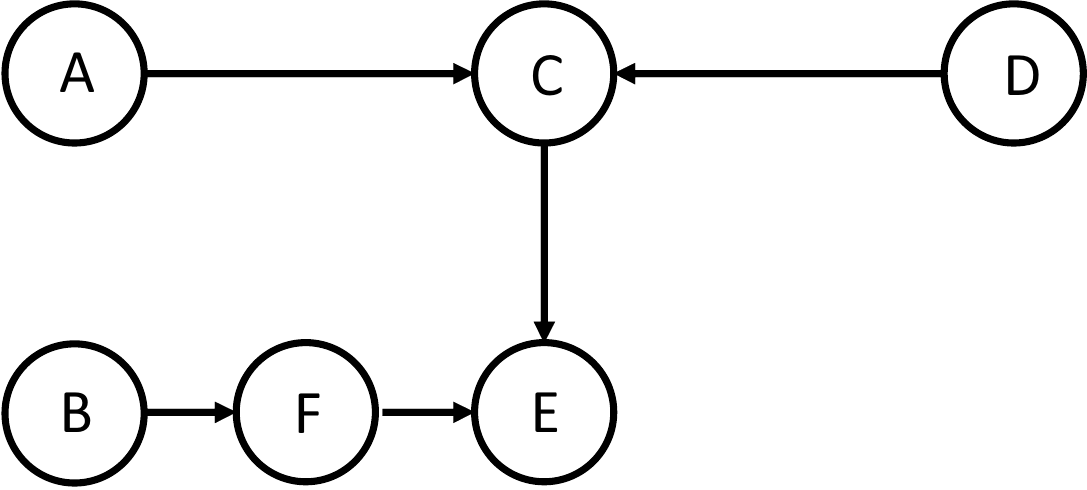}
  \caption{Network for $max$ value function}
  \label{fig:max_with_noise}
\end{figure}
Assume all edge probabilities to be $1$. Now consider two seed allocations $\mathbf{S}^1 = \{(A,j),(B,i),(D,k)\} $ and $\mathbf{S}^2 = \{(A,i), (A,j),(B,i), (D,k)\}$. 

Let the price and value of the items be as follows

\begin{align*}
\val(i) = 4, & \price(i) =1 \\
\val(i) = j, & \price(i) =2 \\
\val(i) = 5, & \price(i) =1 \\
\end{align*}

We assume that when there is a tie in the utility then item higher in the alphabetical order is preferred. Now to restrict the randomness, we set noises for all user item pairs are zero, except $(C,j)$. Depending on this $\noise(C,j)$, there are two classes of possible inner worlds. When $\noise(C,j) > 2$ we refer to the class as $\mathbf{W}_1$, and $\mathbf{W}_2$ corresponds to the class where $\noise(C,j) \leq 2$. As can be seen when $\noise(C,j) > 2$, monotonicity does not hold. Moreover this corresponds to an inner world of class $\mathbf{W}_1$. Thus for all inner world in class $\mathbf{W}_1$, monotonicity does not hold (by definition of equivalent classes in section \ref{sec:eqpw}).

For class $\mathbf{W}_2$ the adoption is indifferent to seeds, i.e. the final adoption of item $i$ does not change after increasing the seed size. Thus with $\mathbf{W}_1$ we have a reduction and with $\mathbf{W}_2$ we have indifference in adoption of $i$. Since these are the only two possible classes of inner worlds, no matter what be the exact distribution of $\noise(C,j)$, the expected adoption is still non-monotone.

\end{proof}

\begin{theorem}\label{thm:monotone_nonmonotone}
Adoption is not self monotone under no noise, when the value function is monotone.
\end{theorem}

\begin{proof}

Consider theorem \ref{thm:val_nonmonotone} and the corresponding utility order. Here we show that same utility order can be obtained when value is supposed to be monotone, by carefully choosing the price terms. Here is the concrete instantiation of the values and prices.\\
Let price of all items be $2$. $\val(k) = 1$, $\val(i) = \val(j) = 20$. $\val(j,k)= 25$, $\val(i, k) = 23.5$. $\val(i, j) = 24$. $\val(i,j,k) = 25$. The deterministic utilities in decreasing order are as follows:\\
$\util^D(j,k) = 25 - 2 - 2 = 21$.\\
$\util^D(i,j) = 24 - 2 - 2 = 20$.\\
$\util^D(i,k) = 23.5 - 2 - 2 = 19.5$.\\
$\util^D(i,j,k) = 25 - 2 - 2 -2 = 19$.\\
$\util^D(j) = \util^D(i) = 20 - 2 = 18$.\\
$\util^D(k) = 1 - 2 = -1$.\\

\end{proof}

\begin{theorem}\label{thm:val_nonmonotone}
Expected adoption is not self monotone under local noise, for an $sup$ value function.
\end{theorem}

\begin{proof}
Consider figure \ref{fig:non_monotone} again. Let there be two items in propagation, $i$ and $j$. We assume the following value and price function.

\begin{align*}
\val(i) = 3 & \price(i) =2 \\
\val(j) = 4 & \price(j) =2 \\
\val(i,j) = 7
\end{align*}

Consider the two seed allocations

\end{proof}
